# Supplementary material for: Learning Gaussian Policies from Corrective Human Feedback
Source: arXiv:1903.05216 source file (2019-03-12)
Supplement: Supplementary file 1 [file supplement.tex]

\appendix
\section{SUPLEMENTARY MATERIAL}
\subsection{BENCHMARKS}\label{sec:benchmarks}
                The first experiment entails the application of \ac{GPC} to the problem of balancing an Underactuated Inverted Pendulum in its unstable equilibrium (most left in \fref{fig:envs}). The environment has $3$ continuous states, chosen by $\textbf{s} = [\cos(\theta),\sin(\theta),\dot{\theta}]$, and $1$ input, which is the torque exerted on the pendulum. The time-limit is set to $200$ timesteps and the costs per time-step are composed of deviations from the reference position and velocity, and an actuation penalty.                
                
                The second experiment is performed in the Cart-Pole domain (middle in \fref{fig:envs}). This environment counts $4$ states and is chosen by  $\textbf{s} = [p,\dot{p},\theta,\dot{\theta}]$, where $p \in [-2.4;2.4]$ denotes the position and $\theta \in [-\frac{1}{12}\pi,\frac{1}{12}\pi]$ the angle of the pole. The action $u \in [-10,10] N$ denotes the force exerted on the cart. An episode is terminated for reaching the state boundaries or by reaching a time-limit of $2500$. Reward is accumulated for $1$ per time-step.

                The final tests concern the exploitation of the Lunar Lander environment (right in \fref{fig:envs}). This environment entails $8$ states, consisting of both continuous (position and velocity) and binary values (ground contact). Actuation is performed using $2$ actions: the main booster for gaining altitude and the side booster for sideways translation and rotation. An episode is terminated for landing or crashing the space-ship, rewarded as 100 or -100 respectively. An efficient approach of the landing site yields an additional 100 to 140 reward. The return is discounted by the action costs.
